# Supplementary material for: LongPerceptualThoughts: Distilling System-2 Reasoning for System-1 Perception
Source: arXiv:2504.15362 source file (2025-04-21)
Supplement: Supplementary file 1 [file appendix-prompt-train-mcqs.tex]

\begin{figure*}[t]
\centering   
\begin{tcolorbox}
\begin{Verbatim}[breaklines=true, commandchars=\\\{\}]
System: XXX
User: <image>\textcolor{red}{[QUESTION]}
Select from the following choices.
\textcolor{red}{[CHOICES]}
Assistant: XXX
\end{Verbatim}
\end{tcolorbox}
\caption{\textbf{Training prompt for DOCCI multi-choices questions.}\AL{need some help}}\label{fig:prompt-train-mcqs}
\end{figure*}
