# Supplementary material for: LongPerceptualThoughts: Distilling System-2 Reasoning for System-1 Perception
Source: arXiv:2504.15362 source file (2025-04-21)
Supplement: Supplementary file 3 [file appendix-table-high-res-docci-variants.tex]

\begin{table}[t]
\centering
\resizebox{\textwidth}{!}{%
\begin{tabular}{@{}l
>{\columncolor[HTML]{EFEFEF}}r rrrrrrr@{}}
\toprule
Model                  & \multicolumn{1}{c}{\cellcolor[HTML]{EFEFEF}Avg} & \multicolumn{1}{c}{V$^{*}$ Bench} & \multicolumn{1}{c}{RealWorldQA} & \multicolumn{1}{c}{MME-RealWorld} & \multicolumn{1}{c}{MMStar} & \multicolumn{1}{c}{MMVP} & \multicolumn{1}{c}{NaturalBench} & \multicolumn{1}{c}{CV bench} \\ \midrule
Qwen2.5-VL-7B-Instruct &                                                     &                             &                                 &                                   &                            &                          &                                  &                              \\
DOCCI-captions         &                                                     &                             &                                 &                                   &                            &                          &                                  &                              \\
DOCCI-MCQ              &                                                     &                             &                                 &                                   &                            &                          &                                  &                              \\
DOCCI-R1-CoT-SFT       &                                                     &                             &                                 &                                   &                            &                          &                                  &                              \\
DOCCI-R1-CoT-DPO       &                                                     &                             &                                 &                                   &                            &                          &                                  &                              \\
DOCCI-R1-CoT-SFT-then-DPO       &                                                     &                             &                                 &                                   &                            &                          &                                  &                              \\ \bottomrule
\end{tabular}%
}
\caption{\textbf{Comparison of models trained on different DOCCI~\cite{} derived datasets at higher resolution $2048 \times 2048$.}}
\label{tab:my-table}
\end{table}
